# Supplementary material for: Debiasing Sentence Embedders through Contrastive Word Pairs
Source: arXiv:2403.18555 source file (2024-03-27)
Supplement: Supplementary file 1 [file appendix.tex]

In this section we provide a List of contrastive debiasing terms and a list of sentences used in the experiments.

\newpage
\subsection*{List of contrastive debiasing terms}
\begin{table}[h!]
\caption{\label{tab:conwords} List of contrastive debiasing terms used in the experiments.} %TODO cite bolukbasi implementation as source
\begin{tabular}{|cc|}
\hline
female & male \\
women & men \\
girl & boy \\
she & he \\
actress & actor \\
heroine & hero \\
mother & father \\
lady & gentleman \\
queen & king \\
sister & brother \\
her & him \\
\hline
\end{tabular}

\end{table}

\subsection*{List of neutral sentences}
\begin{table}[h!]
\caption{\label{tab:neutralsent} List of neutral sentences used in the experiments.} 
\begin{tabular}{|c|}
\hline
I am a [BLANK]\\
I work as a [BLANK]\\
My occupation is [BLANK]\\
My dream job is  [BLANK]\\
works as a  [BLANK]\\
wants to become a  [BLANK]\\
Overall i am quite happy with being a [BLANK] \\
I am depressed working as a [BLANK] \\
In conclusion i am neutral towards my job as a [BLANK] \\
I am working as a [BLANK] \\
This is my job: [BLANK]\\
I am conflicted about being a [BLANK]\\
\hline
\end{tabular}

\end{table}
